# Supplementary material for: Transfer Learning of Graph Neural Networks with Ego-graph Information Maximization
Source: arXiv:2009.05204 source file (2021-10-26)
Supplement: Supplementary file 1 [file appendix.tex]

\documentclass{article}

% if you need to pass options to natbib, use, e.g.:
%     \PassOptionsToPackage{numbers, compress}{natbib}
% before loading neurips_2021

% ready for submission
\usepackage{neurips_2021}

% to compile a preprint version, e.g., for submission to arXiv, add add the
% [preprint] option:
%     \usepackage[preprint]{neurips_2021}

% to compile a camera-ready version, add the [final] option, e.g.:
%     \usepackage[final]{neurips_2021}

% to avoid loading the natbib package, add option nonatbib:
%    \usepackage[nonatbib]{neurips_2021}

\usepackage[utf8]{inputenc} % allow utf-8 input
\usepackage[T1]{fontenc}    % use 8-bit T1 fonts
\usepackage{hyperref}       % hyperlinks
\usepackage{url}            % simple URL typesetting
\usepackage{booktabs}       % professional-quality tables
\usepackage{amsfonts}       % blackboard math symbols
\usepackage{nicefrac}       % compact symbols for 1/2, etc.
\usepackage{microtype}      % microtypography
\usepackage{xcolor}         % colors
\usepackage{amsmath, amsfonts, amssymb, xspace, color, amsbsy, caption, adjustbox, amsthm}
\usepackage{tabularx}
\usepackage{tikz, graphicx}
\usepackage{enumitem}
\usepackage{multirow}
\usepackage{cleveref}
\usetikzlibrary{positioning}
\usepackage[linesnumbered,ruled,lined]{algorithm2e}
\usepackage[font=small,labelfont=bf]{caption}
\usepackage{subcaption}
%,labelfont=bf,textfont=bf
\usepackage{esvect}

\usepackage{changepage}
\usepackage{pifont}
\theoremstyle{plain}

\newtheorem{thm:eg}{Example}
%\newtheorem{lemma}[theorem]{Lemma}

% ----------------------------------------------------------------------
% For draft editing.
% ----------------------------------------------------------------------

% \newcommand{\hide}[1]{} %hide

 % a new paragraph without indent

% ----------------------------------------------------------------------
%  Common abbreviations and words with accents
% ----------------------------------------------------------------------

 % and others
 % that is
 % for example
 % that is
 % with respect to

 % and others
 % and others

% ----------------------------------------------------------------------
% Math symbols.
% ----------------------------------------------------------------------

 % Cheap displaystyle operators

			% use instead of $|x|$
			% use instead of $\|x\|$

% ----------------------------------------------------------------------
% Document-specific commands.
% ----------------------------------------------------------------------

% Shrink space.
% \setlength{\floatsep}{4pt plus 4pt minus 1pt}
% \setlength{\textfloatsep}{4pt plus 2pt minus 2pt}
% \setlength{\intextsep}{4pt plus 2pt minus 2pt}

% \setlength{\dbltextfloatsep}{3pt plus 2pt minus 1pt}
% \setlength{\dblfloatsep}{3pt plus 0pt minus 0pt}

% \setlength{\abovedisplayskip}{2pt plus 1pt minus 1pt}
% \setlength{\belowdisplayskip}{2pt plus 1pt minus 1pt}

% ----------------------------------------------------------------------
% Commands used in clustering.
% ----------------------------------------------------------------------

\SetKwRepeat{Do}{do}{while}
\title{Formatting Instructions For NeurIPS 2021}

% The \author macro works with any number of authors. There are two commands
% used to separate the names and addresses of multiple authors: \And and \AND.
%
% Using \And between authors leaves it to LaTeX to determine where to break the
% lines. Using \AND forces a line break at that point. So, if LaTeX puts 3 of 4
% authors names on the first line, and the last on the second line, try using
% \AND instead of \And before the third author name.

\author{%
  David S.~Hippocampus\thanks{Use footnote for providing further information
    about author (webpage, alternative address)---\emph{not} for acknowledging
    funding agencies.} \\
  Department of Computer Science\\
  Cranberry-Lemon University\\
  Pittsburgh, PA 15213 \\
  \texttt{hippo@cs.cranberry-lemon.edu} \\
  % examples of more authors
  % \And
  % Coauthor \\
  % Affiliation \\
  % Address \\
  % \texttt{email} \\
  % \AND
  % Coauthor \\
  % Affiliation \\
  % Address \\
  % \texttt{email} \\
  % \And
  % Coauthor \\
  % Affiliation \\
  % Address \\
  % \texttt{email} \\
  % \And
  % Coauthor \\
  % Affiliation \\
  % Address \\
  % \texttt{email} \\
}

\begin{document}

%%%%%%%%%%%%%%%%%%%%%%%%%%%%%%%%%%%%%%%%%%%%%%%%%%%%%%%%%%%%

\appendix

\input{supps/proof}
\input{supps/method_supps}
\input{supps/experiment_supps}

\bibliography{ref}
\bibliographystyle{plain}

\end{document}
