# Supplementary material for: Transfer Learning of Graph Neural Networks with Ego-graph Information Maximization
Source: arXiv:2009.05204 source file (2021-10-26)
Supplement: Supplementary file 2 [file macro.tex]

\usepackage{amsmath, amsfonts, amssymb, xspace, color, amsbsy, caption, adjustbox, amsthm}
\usepackage{tabularx}
% \usepackage{tikz, graphicx, algorithmic, capt-of, ifthen, calc, algorithm}
\usepackage{tikz, graphicx}
\usepackage{enumitem}
\usepackage{multirow}
\usepackage{cleveref}
%\usepackage{subfig}
\usetikzlibrary{positioning}
\usepackage[linesnumbered,ruled,lined]{algorithm2e}
\usepackage[font=small,labelfont=bf]{caption}
\usepackage{subcaption}
%,labelfont=bf,textfont=bf
\usepackage{esvect}

\usepackage{changepage}
\usepackage{pifont}
%\theoremstyle{definition}
\theoremstyle{plain}
\newtheorem{definition}{Definition}[section]
\newtheorem{theorem}{Theorem}[section]
\newtheorem{corollary}{Corollary}[theorem]
\newtheorem{lemma}[theorem]{Lemma}
\newtheorem{thm:eg}{Example}
%\newtheorem{lemma}[theorem]{Lemma}
\newtheorem{remark}{Remark}

\newcommand{\Ours}{\textsc{Egi}\xspace}
\newcommand{\xhdr}[1]{\vspace{1.7mm}\noindent{{\bf #1}}}
\newcommand{\tick}{\ding{52}}
% ----------------------------------------------------------------------
% For draft editing.
% ----------------------------------------------------------------------

\newcommand{\red}[1]{\textcolor{red}{#1}}
\newcommand{\blue}[1]{\textcolor{blue}{#1}}
% \newcommand{\hide}[1]{} %hide
\newcommand{\vpara}[1]{\vspace{0.01in}\noindent\textbf{#1}}
\newcommand{\para}[1]{\vspace{0.1in}\noindent\textbf{#1}}
\newcommand{\pa}[2]{\vspace{#1}\noindent\textbf{#2}} % a new paragraph without indent
\newcommand{\benum}[1]{\begin{enumerate}#1\end{enumerate}}
\newcommand{\bitem}[1]{\begin{itemize}#1\end{itemize}}

\newcommand{\ulpara}[1]{\vspace{0.01in}\noindent\emph{#1}}

% ----------------------------------------------------------------------
%  Common abbreviations and words with accents
% ----------------------------------------------------------------------

\newcommand{\etal}{\emph{et~al.}\xspace} % and others
\newcommand{\ie}{\emph{i.e.}\xspace} % that is
\newcommand{\eg}{\emph{e.g.}\xspace} % for example
\newcommand{\etc}{\emph{etc.}\xspace} % that is
\newcommand{\wrt}{\emph{w.r.t.}\xspace} % with respect to
\newcommand{\iid}{\emph{i.i.d.}\xspace}

\newcommand{\naive}{na\"{\i}ve\xspace} % and others
\newcommand{\Naive}{Na\"{\i}ve\xspace} % and others
\newcommand{\ssym}{§}

% ----------------------------------------------------------------------
% Math symbols.
% ----------------------------------------------------------------------

\newcommand{\beal}[1]{\begin{align}#1\end{align}}
\newcommand{\beq}[1]{\begin{equation}#1\end{equation}}
\newcommand{\beqn}[1]{\begin{eqnarray}#1\end{eqnarray}}

\newcommand{\Sum}{\sum\limits} % Cheap displaystyle operators
\newcommand{\Max}{\max\limits}
\newcommand{\Min}{\min\limits}
\newcommand{\Prod}{\prod\limits}
\newcommand{\Lim}{\lim\limits}
\newcommand{\Bcup}{\bigcup\limits}

\newcommand{\abs}[1]{\mathopen| #1 \mathclose|}			% use instead of $|x|$
\newcommand{\norm}[1]{\mathopen\| #1 \mathclose\|}			% use instead of $\|x\|$
\newcommand{\inner}[2]{\langle #1, #2 \rangle}

\DeclareMathOperator*{\argmax}{argmax}
\DeclareMathOperator*{\argmin}{argmin}

\def \E {\mathrm{E}}

\def \c {\mathbf{c}}
\def \d {\mathbf{d}}
\def \e {\mathbf{e}}
\def \f {\mathbf{f}}
\def \g {\mathbf{g}}
\def \h {\mathbf{h}}
\def \l {\mathbf{l}}
\def \m {\mathbf{m}}
\def \o {\mathbf{o}}
\def \p {\mathbf{p}}
\def \q {\mathbf{q}}
\def \r {\mathbf{r}}
\def \t {\mathbf{t}}
\def \u {\mathbf{u}}
\def \v {\mathbf{v}}
\def \w {\mathbf{w}}
\def \x {\mathbf{x}}
\def \y {\mathbf{y}}
\def \z {\mathbf{z}}
\def \A {\mathbf{A}}
\def \H {\mathbf{H}}
\def \I {\mathbf{I}}
\def \L {\mathbf{L}}
\def \P {\mathbf{P}}
\def \U {\mathbf{U}}
\def \W {\mathbf{W}}

\def \B {\mathcal{B}}
\def \C {\mathcal{C}}
\def \D {\mathcal{D}}
\def \F {\mathcal{F}}
\def \M {\mathcal{M}}
\def \N {\mathcal{N}}
\def \O {\mathcal{O}}
\def \Q {\mathcal{Q}}
\def \R {\mathcal{R}}
\def \S {\mathcal{S}}
\def \T {\mathcal{T}}
\def \calX {\mathcal{X}}
\def \calY {\mathcal{Y}}
\def \calH {\mathcal{H}}
\def \calL {\mathcal{L}}

\def \X {\mathbf{X}}
\def \Y {\mathbf{Y}}
\def \Z {\mathbf{Z}}

\def \RR {\mathbb{R}}
\def \NN {\mathbb{N}}
\def \SSS {\mathbb{S}}
\def \regret {\mbox{regret}}
\def \Uh {\widehat{U}}

\def \sig {\sigma}
\def \gt {g_{\theta}}
\def \gi  {g_i}
\def \gid {g_{i'}}
\def \fj  {f_{j}}
\def \fjd {f_{j'}}

% ----------------------------------------------------------------------
% Document-specific commands.
% ----------------------------------------------------------------------
\newcommand{\ADD}[1]{\textcolor{red}{Added: #1}}
\newcommand{\DEL}[1]{\textcolor{blue}{Deleted: #1}}
\newcommand{\QZ}[1]{\textcolor{orange}{Bran: #1}}
\newcommand{\carl}[1]{\textcolor{purple}{Carl: #1}}


\def \zero {\mathbf{0}}
\def \one {\mathbf{1}}
\def \PT {\mathbf{P}^\text{T}}

\newcommand{\hop}{\texttt{Hop}\xspace}
\newcommand{\SP}{\texttt{SP}\xspace}
\newcommand{\RWR}{\texttt{RWR}\xspace}
\newcommand{\wave}{\textsc{Wavelet}\xspace}
\newcommand{\our}{\textsc{AFGRE}\xspace}
\newcommand{\iknn}{\textsc{Ink}\xspace}
\newcommand{\knn}{top-$k$\xspace}
\newcommand{\rd}[1]{^{(#1)}}
\newcommand{\lb}[1]{\underline{#1}\xspace}
\newcommand{\ub}[1]{\overline{#1}\xspace}


% Shrink space.
% \setlength{\floatsep}{4pt plus 4pt minus 1pt}
% \setlength{\textfloatsep}{4pt plus 2pt minus 2pt}
% \setlength{\intextsep}{4pt plus 2pt minus 2pt}

% \setlength{\dbltextfloatsep}{3pt plus 2pt minus 1pt}
% \setlength{\dblfloatsep}{3pt plus 0pt minus 0pt}

% \setlength{\abovedisplayskip}{2pt plus 1pt minus 1pt}
% \setlength{\belowdisplayskip}{2pt plus 1pt minus 1pt}


% ----------------------------------------------------------------------
% Commands used in clustering.
% ----------------------------------------------------------------------


\def \Kappa {\boldsymbol{\kappa}}
\def \sS {\mathbf{S}}
\def \sX {\mathcal{X}}
\def \sz {\mathcal{Z}}
\def \Mu {\boldsymbol{\mu}}
\def \Eta {\boldsymbol{\eta}}
\def \vmf {\mathbf{vMF}}
\def \cluster {\textsc{Shifting-Window Clustering }}

\SetKwRepeat{Do}{do}{while}
